# Supplementary material for: Unveiling A Hidden Risk: Exposing Educational but Malicious Repositories in GitHub
Source: arXiv:2403.04419 source file (2024-03-07)
Supplement: Supplementary file 1 [file 080appendix.tex]

%%%%%%%%%%%%%%%%%%%%%%%%%%%%%%%%%%%%%%%
% AUTHOR: Christos Faloutsos
% INSTITUTION: CMU
% DATE: April 2019
% GOAL: to streamline the paper presentations
%%%%%%%%%%%%%%%%%%%%%%%%%%%%%%%%%%%%%%%

\section{Stealth appendix}
\reminder{[here we put self notes etc, that we will NOT include
in the final paper]}
